# Supplementary material for: Measurement of isotopic separation of argon with the prototype of the cryogenic distillation plant Aria for dark matter searches
Source: arXiv:2301.09639 source file (2023-01-26)
Supplement: Supplementary file 1 [file appendix.tex]

\section{Universal Gas Analyzer (UGA)}
\label{appa}

\begin{figure}[htbp]
\centering
\includegraphics[width=\columnwidth]{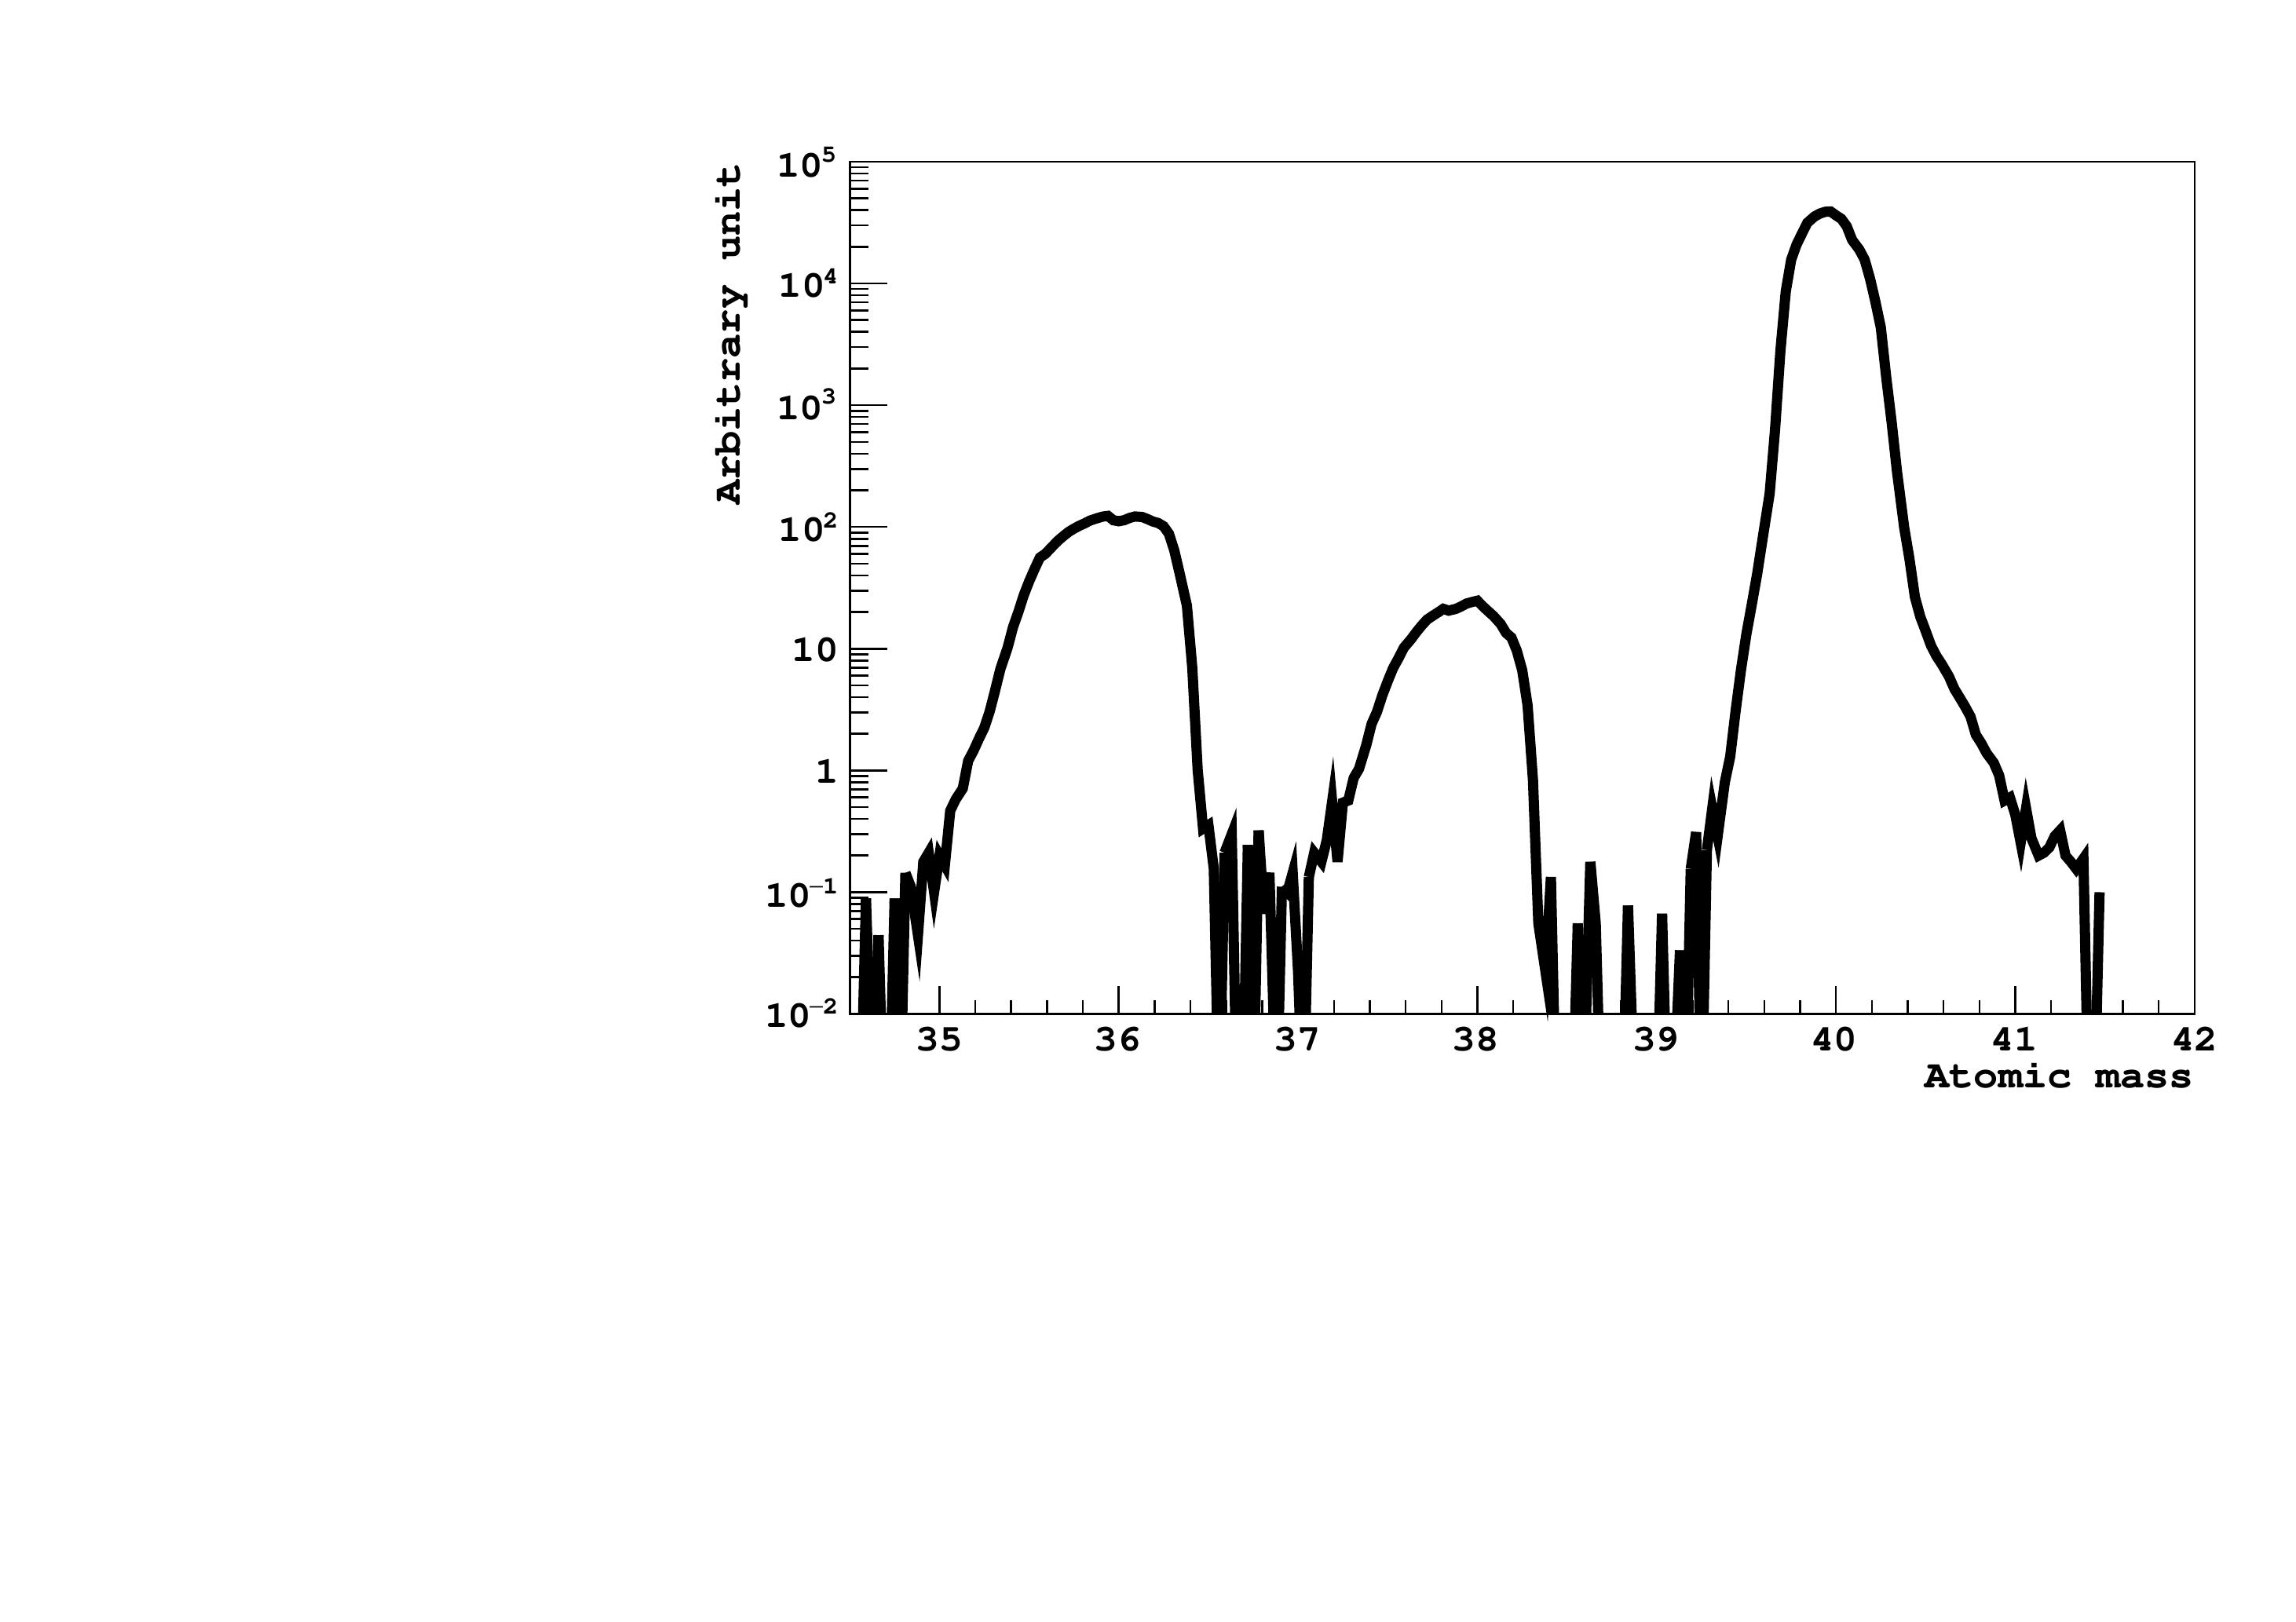}
\caption{Example of a spectrum obtained by UGA during the run in spectrum mode. Pressure in mbar in log scale as a function of the atomic mass. Closeup of all the values near the argon peaks.}
\label{Spettro} 
\end{figure}
From here begins a process within the UGA through the joint use of Bypass Valve and Turbo Pump which leads to a significant reduction in gas pressure, up to the order of $10^{-7}$ mbar required by the RGA. 
When neutral gas molecules enter the RGA they pass through an ionization region. A hot cathode (also known as a filament) emits electrons that collide with the molecules we want to study and ionize them (with single or double ionization). At this point, the gas has been ionized and has a certain $e/m$ ratio, concerning which we can distinguish gases with different masses. Subsequently, an electrostatic lens accelerates them before they enter a quadripole. This deflects the various gases in different ways according to the $e/m$ ratio; only particles with a certain radius will reach the next detector and therefore an electrical signal proportional to the number of particles with a certain ratio $e/m$ will be recorded; this selection is possible thanks to a successive lens system known as $V-Lens$\texttrademark. This procedure is then repeated for different trays (and therefore different values of the ratio) until the whole spectrum is reconstructed. Finally, detection is made possible thanks to a Faraday cup and a Multiplier detecting and amplifying the charge of the ions. In addition, the UGA has an internal stove that maintains high temperatures ($80$ C ° -$100$C °). In this way, the internal temperature will be constant and stable and this is useful to avoid discrepancies in the gas detection. \\
In the spectra in figure (\ref{Spettro}), the reciprocal of the $e/m$ ratio is present along the x-axis, having assumed $ e = 1 $. This means that in the case of double ionization there will be an additional peak caused by a given gas. For example, \ce{^40Ar} shows a peak for $ m = 40 $ in case of single ionization and $ m = 20 $ in case of double ionization. Before proceeding with the calibration it is necessary to perform the instrument tuning. The first step in tuning consists of identifying the exact position of each peak as there could be an offset between the real mass and the peak position. The peaks are therefore translated in such a way as to be positioned in correspondence with the desired mass. \\
Subsequently, it is required to optimize the following values:
\begin{enumerate}
    \item{\emph{Emission current} is the current of the electron emitted by the filament. The higher the current, the higher the filament temperature.}
    \item{\emph{Electron Energy} is the accelerating voltage between the filament and the ion source. It is the energy that the electrons will have in the ion source.}
    \item{\emph{Ion energy}. Is the energy voltage of the ion source and the energy that the ions will have when emitted. }
    \item{\emph{Extraction Voltage}. Is the voltage of ion extraction in the ion source.}
\end{enumerate}
The tuning parameters used during our experiment are in the following table. 
\begin{table}[ht]
\centering
\begin{tabular}{c c c }
\hline\noalign{\smallskip}
Tuning parameter&Range & Value chosen \\
\noalign{\smallskip}\hline\noalign{\smallskip}
Emission&$0-5$ mA&$1$ mA\\ 
Electron Energy&$0-100$ eV&$40$ eV\\ 
Ion Energy &$0-10$ eV&$10$ eV\\ 
Extract&$0-130$ V &$20$ V\\ 
\hline
\end{tabular}
\caption{Tuning parameter allowed range and values chosen for the data taking.}
\end{table}
The calibration of the instrument consists of finding the correct value of the \emph{Electronic Gain} (mbar/mA), that is the value that allows transforming mA into mbar along the y-axis. We sampled free air by disconnecting the UGA capillary and observed the nitrogen peak. We have therefore modified the aforementioned parameter so that the peak settles at a pressure of $780$ mbar (i.e. the atmospheric pressure multiplied by the percentage of nitrogen in the air). 
Since the capillary system is made in such a way that the pressure reaching the UGA is always in the order of the atmospheric one, we expect the partial pressure values measured in the graphs to be quite reliable. However, the response of the device, intended as the current recorded concerning the number of charged particles with a given $e / m$ ratio, is not always the same. Therefore the calibration is not intended for the whole spectrum but for one peak at a time. This explains why in the previous graphs (\ref{Spettro}) the total pressure appears significantly higher than the atmospheric one. This could invalidate the measurement of the relationship between \ce{^36Ar} and \ce{^40Ar} but certainly not $S_{T-B, 36-40}$. This happens because the separation is given by the ratio between the concentrations, and therefore any multiplying factors simplify and eliminate each other.
\section{Plant operations}
\label{appb}
\begin{figure}[htbp]
\centering
\includegraphics[height=6.5cm, width=8cm]{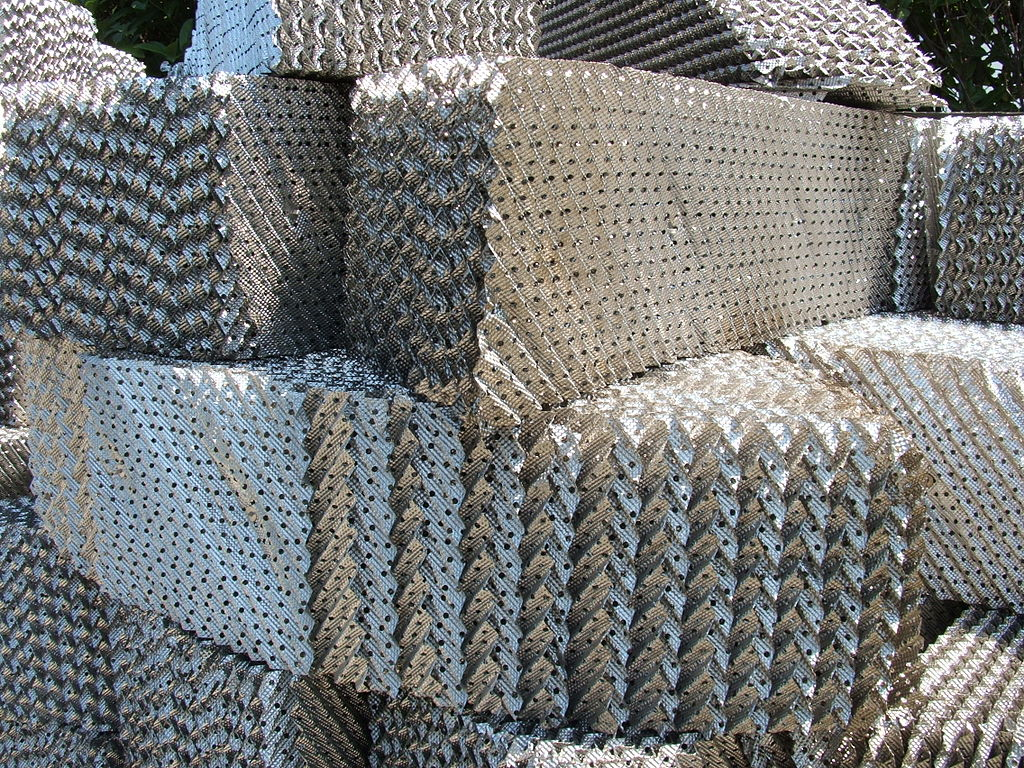}
\caption{Packing metal gauze Sulzer CY}
\label{packing}
\end{figure}

\subsection{Description of mass transfer}
In a column with structured packing (also called a packed column), the mass transfer occurs through the counter-current flow of the liquid (which descends by gravity) with the vapor (which rises). Column efficiency is commonly expressed as the height of the bed or plate that generates a composition variation equivalent to that of a theoretical plate (HETP). HETP is an empirical parameter that allows designers to estimate the height of the packed plate based on the number of theoretical equilibrium stages. The use of simulations that exploit the equilibrium stages represents a consolidated calculation methodology available in commercial software packages.
The exercise phase is used to validate the HETP estimated at the design stage. The analysis of the results of this part is reported in section \ref{Results}. The mass transfer efficiency is expected to depend on the geometry of the packing, the hydraulic conditions, the physical properties, and the thermodynamic behavior of the system.

\subsection{Description of column's operation}
In this type of column, the liquid deriving from the condensation of the process fluid, which enters the column as reflux, is sprayed from above and descends by gravity, distributing itself on the packing, where it encounters a more or less pronounced resistance caused by the vapor current that it goes up the column through the packed bed.
The main purpose of distillation equipment is to establish intimate contact between rising vapor and descending liquid; this contact is physically achieved by the gauze structured packing.
The exchanges of heat and matter between the liquid and vapor streams that move in countercurrent through the packed bed of the column occur as a result of the differences in thermodynamic parameters such as concentration, temperature, and pressures between the fluids themselves. Such exchanges take place, all other conditions being equal, to a greater extent the longer the liquid-vapor contact time.
In a structured packed column, the vapor laps around the liquid rather than bubbling through it as it does in plate columns and this involves a lower pressure drop. A higher pressure drop results in higher pressure and, consequently, a higher temperature at the bottom of the column. If excessive, this difference can adversely affect the separation (reduced relative volatility).
To ensure that there is an efficient liquid-vapor exchange, it is necessary to distribute the liquid as evenly as possible over the entire section of the packing; complete irrigation of the exchange surface is a prerequisite for correct operation. It should be added that the structured packing can create preferential paths for the liquid and for the vapor which can cause a decrease in the efficiency of the exchange of matter between the two phases.
To cope with this situation, the element that guarantees the uniform distribution of the liquid is the distributor.
The effect of the decrease in efficiency caused by the poor distribution of liquids tends to manifest itself with increasing bed depth, consequently, the height of the bed is usually limited to a height equivalent to a certain number of theoretical plates.
In our specific case, about $25$, corresponds to a packing section height of $2.56$ m. The liquid coming out of a packing section must be collected and mixed thoroughly before passing to the distributor of the bed below.
\subsection{Distributor construction details}
The prerequisite for the correct functioning of the packed beds is an adequate quality of the initial distribution of the liquid. This means using a dispenser with a sufficient and evenly distributed irrigation point density. 
The distributors used in the Aria column were patented by the Polaris company which also designed and built the entire system (\ref{Distributor}).
These distributors are characterized by seven channels for the passage of steam (length $125$ mm, diameter $42$ mm) and $12$ channels for the passage of liquid (length $100$ mm and $8$ mm in diameter, equipped with three $3$ mm holes placed at one height of $30$, $40$, and $50$ mm for the percolation of the liquid into the underlying layer).
The liquid descends from above and is collected in the dispenser plate, as soon as the liquid level on this plate reaches the height of the first hole, it begins to leach into the level below. If the amount of liquid is sufficient to reach the height of the third hole, the liquid will percolate from all three holes.
\subsection{Packing construction details}
\begin{figure}[htbp]
\centering
\includegraphics[height=4.5cm, width=8cm]{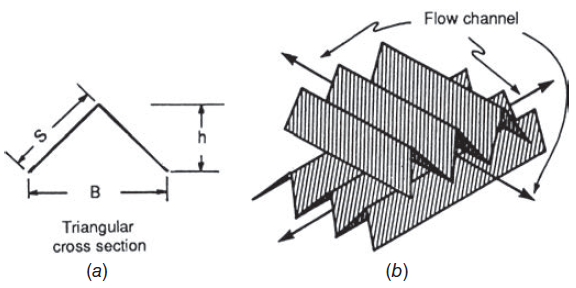}
\caption{Crimp geometry in structured packings. (a) Flow channel cross-section. (b) Flow channel arrangement.}
\label{Crimp_geometry}
\end{figure}
The structured packing has a well-defined geometric structure, which consists of an alternating arrangement of corrugated sheets that form intersecting open channels for the flow of steam.
The individual layers are produced by a special metallic gauze that maximizes the capillary effect. Therefore, the surface area is wetted with very low liquid loads.
The crimp size defines the opening between adjacent corrugated layers. Smaller B, h and, S produce narrower openings, (hence a larger surface area) per unit of volume and more efficient packing, but greater resistance to gas flow and a lower capacity (understood as the volumetric flow rate of steam).
The angle of inclination of the corrugation and the shape of the corrugation, h and B, strongly influence the pressure drop and the geometric area in which the mass transfer takes place.
Corrugations spread the flow of gas and liquid through a single element in a series of parallel planes. To spread the gas and liquid evenly over all radial planes, adjacent elements are rotated so that the layers (or sheets) of one element is at a fixed angle to the underlying layer (\ref{packed bed}).
\begin{figure}[htbp]
\centering
\includegraphics[height=4.5cm, width=8cm]{images/packed bed.png}
\caption{Example of how the packing layers are assembled.}
\label{packed bed}
\end{figure}
For a good diffusion, the height of the element is relatively small (generally from $200$ to $300$ mm, from $8$ to $12$ inches) and the rotation angle is about $90°$.
The surface is textured to allow for lateral diffusion of the liquid, promote film turbulence and improve the area available for mass transfer.
The packing surfaces contain holes that serve as communication channels between the top and bottom surfaces of each sheet.
In each element, the corrugated sheets are provided with an angle of inclination of approximately $45°$ with respect to the vertical (indicated by the letter Y). This angle is large enough for good liquid drainage, avoiding stagnant pockets and regions of liquid accumulation, and small enough to prevent gas from bypassing metal surfaces.
The thickness of the material defines the vacuum fraction $\epsilon$ $(\mathrm{m}^3/\mathrm{m}^3)$, which typically varies in the range from $0.9$ to $0.98$.
It is characterized by a wettability of $5\%$ Minimum liquid load approx. $0.05$ $(\mathrm{m}^3/\mathrm{m}^2*h)$.
The three main hydraulic performance criteria of the packing are expressed by capacity, pressure drop, and liquid retention.

\section{The simulation program}
\begin{figure}[htbp]
\centering
\includegraphics[height=13.41cm, width=5.18cm]{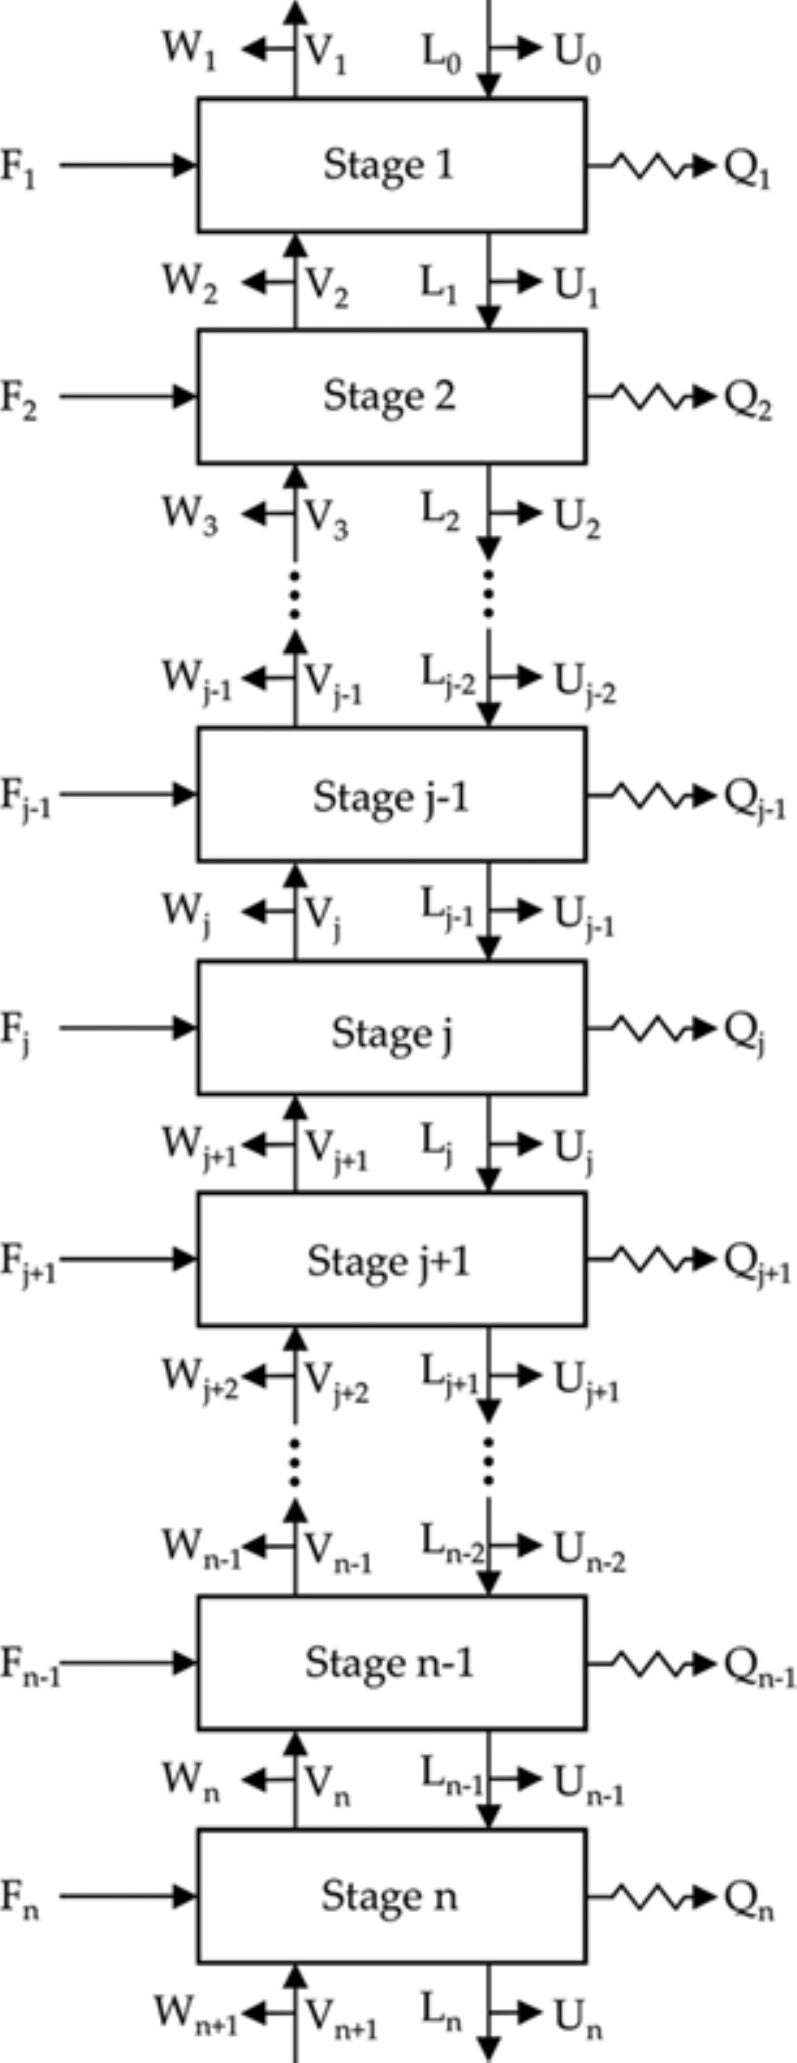}
\caption{The general structure of the stages of a distillation column \cite{Steffen:2017}. $F_j$ is the input mass flow, $W_j$, and $U_j$ represent the heat exchanged between one stage and another, while $Q_j$ is the heat removed or added externally in a stage. $V_j$ and $L_j$ are respectively the vapor and liquid mass flow crossing the column in stage $j$.}
\label{Hysys1}
\end{figure}
\label{appc}
$$ F_j+V_{j+1}+L_{j-1}=V_j+L_j $$
$$ F_j z_j+V_{j+1} y_{j+1}+L_{j-1} x_{j-1}= V_{j} y_{j} + L_{j} x_{j} $$
$$ Q_j+V_{j+1} W_{j+1}+L_{j-1} U_{j-1}=V_{j}W_{j}+L_{j} U_{j}$$
$$ y_{j}= K_{j} x_{j} $$
These equations represent the conservation laws of a generic state $ j $ of a rigorous and binary distillation column.
Where $x_i$, $y_i$, and $z_i$ are the concentrations of the lighter element respectively in liquid, vapor, and mixed states. $K_i$ is the K-value: the ratio between the concentration in the vapor and liquid phase of the same element. HYSYS, performing rigorous calculations, solves a system made of these four equations for each stage of the distillation column, thus the computation time increases considerably within the number of stages $N$. On the other side short-cut methods such as McCabe-Thiele \cite{MCT:2000} are based on the following assumptions:
\begin{enumerate}
    \item {There is only one feeding point, i.e. there are just one stage $\Bar{j}$ such that $F_{\Bar{j}}=F$; for all the others $F_j=0$}
    \item{There is only two extraction point from the top and bottom of the column. The extraction mass flows are respectively called $D$, and $B$.}
    \item{\emph{Constant Molar Overflow}. The mixture has a constant heat of vaporization and heat effects are negligible: the energy balance equation is not taken into account and $$L_1\;=\;L_2\;=\;L_3\;=\;...\;L_j\;=\;L,$$
    $$V_1\;=\;V_2\;=\;V_3\;=\;...\;V_j\;=\;V,$$
    for the rectifying section (above the feeding point), while for the stripping
    $$L_N\;=\;L_{N-1}\;=\;L_{N-2}\;=\;...\;L'_j\;=\;L',$$
    $$V_N\;=\;V_{N-1}\;=\;V_{N-2}\;=\;...\;V'_j\;=\;V'.$$
    }
\end{enumerate}
Thus the balance equations could be rewritten as
$$F=(L'-L)-(V'-V),$$
$$F=B+D,$$
where these two equations are therefore sufficient to describe a binary shortcut column, further details about the demonstrations could be found in (\cite{Distillation:1992}, chapter two). The rules and approximations just explained concern McCabe-Thiele in particular, other shortcut methods may have different conditions.\\ \\
